# Supplementary material for: A Problem-Oriented Perspective and Anchor Verification for Code Optimization
Source: arXiv:2406.11935 source file (2026-02-25)
Supplement: Supplementary file 6 [file instruction_prompt.tex]

\begin{figure}[t]
    \centering
    \begin{tcolorbox}[colframe=lightblue, colback=white, width=0.49\textwidth]
        \begin{minted}[breaklines, fontsize=\footnotesize]{cpp}
Given the program below, improve its performance:

### Program:
{slow_code}

### Optimized Version:
        \end{minted}
    \end{tcolorbox}
    \caption{Instruct Prompt.}
    \label{fig:instruct_prompt}
\end{figure}
